# Supplementary material for: Joint Determination of Reactor Antineutrino Spectra from $^{235}$U and $^{239}$Pu Fission by Daya Bay and PROSPECT
Source: arXiv:2106.12251 source file (2022-02-23)
Supplement: Supplementary file 1 [file Supplemental_README.pdf]

```
import numpy as np
from scipy import interpolate
import matplotlib.pyplot as plt
```

## Supplemental Material Demonstration

---

In this publication supplemental material are provided detailing the jointly unfolded antineutrino spectrum from  $^{235}\text{U}$  along with the  $A_c$  smearing matrix and the covariance matrix containing all uncertainties. In this note we show how these data can be used to compare this measurement to a theoretical model.

### Contents

---

`DayaBay_PROSPECT_JointUnfold_U235_Spectrum.txt` : The unfolded spectrum along with bin edges and bin centers

`DayaBay_PROSPECT_JointUnfold_U235_Covariance.txt` : The covariance matrix containing all uncertainties *except* those related to the unfolding procedure. This matrix can be used in combination with the smearing matrix to compare models or other predictions to the unfolded spectrum.

`DayaBay_PROSPECT_JointUnfold_U235_Smearing_Matrix.txt` : The  $A_c$  smearing matrix as prescribed by the Wiener SVD method. This matrix is applied to external models for comparison to the unfolded spectrum.

`DayaBay_PROSPECT_JointUnfold_Isotope_Covariance_Full.txt` : The full covariance matrix, including unfolding uncertainties, for both  $^{235}\text{U}$  and  $^{239}\text{Pu}$  that should be utilized when using the unfolded spectrum to generate predictions for other experiments. This is a 50x50 matrix that includes both the individual uncertainties and the isotopic correlations.

### Reading supplemental data

---

The data are provided in comma-separated tabular data. This can be read using the `numpy.loadtxt` function or any similar parser.

```
bin_low, bin_centers, bin_high = np.loadtxt('./DayaBay_PROSPECT_JointUnfold_U235_Spectrum.txt',
                                             usecols=(0,1,2), unpack=True)
bin_edges = np.concatenate((bin_low, bin_high[-1:]))

spectrum = np.loadtxt('./DayaBay_PROSPECT_JointUnfold_U235_Spectrum.txt', usecols=3)

a_c = np.loadtxt('./DayaBay_PROSPECT_JointUnfold_U235_Smearing_Matrix.txt')

covariance = np.loadtxt('./DayaBay_PROSPECT_JointUnfold_U235_Covariance.txt')

full_covariance = np.loadtxt('./DayaBay_PROSPECT_JointUnfold_Isotope_Covariance_Full.txt')
```

### Visualizing the data

---

#### Plotting the spectrum

Here we plot the jointly unfolded spectrum with visual errorbars generated from the diagonal elements of the covariance matrix. These errors are meant as a guide and do not capture the full uncertainties, which include correlated uncertainties from experimental methods and from the unfolding procedure.

```

errorBars = np.sqrt(np.diagonal(covariance))

plt.errorbar(bin_centers, spectrum, yerr=errorBars,
             marker='.', linestyle='None', label='Joint Unfolded')
plt.xlabel('Neutrino Energy [MeV]');
plt.ylabel('Flux x 1e-43');
plt.legend(frameon=True);
plt.ylim(0,2);

```

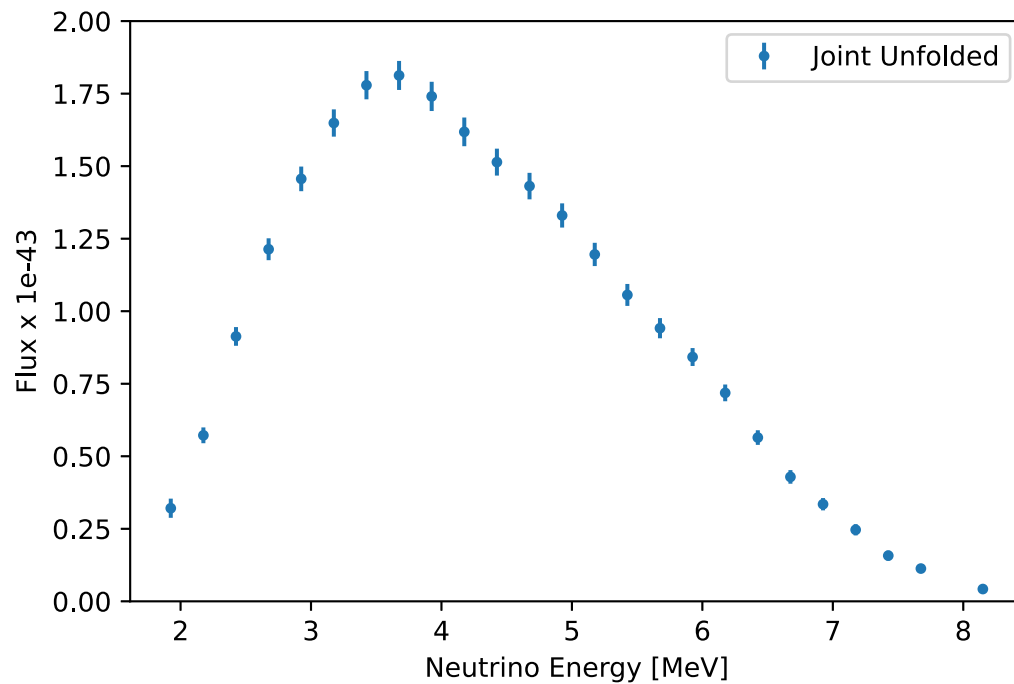

## The smearing matrix

The  $A_c$  smearing matrix is shown below. This matrix contains all the impact from the unfolding process and must be used to compare the result to other measurements or models.

```

plt.imshow(a_c, origin='lower')
plt.colorbar();

```

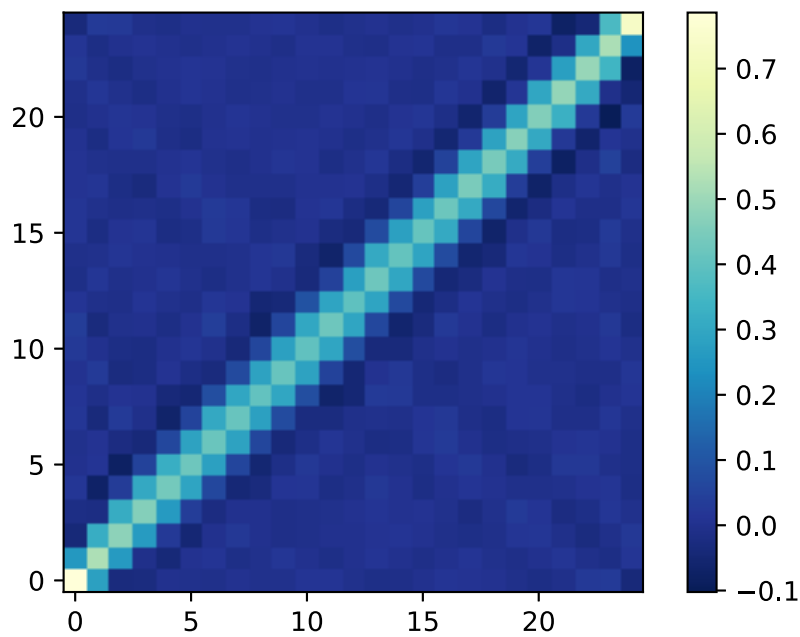

## Comparing the covariance matrices

The analysis produces two slightly different covariance matrices. The first is generated analytically and contains all the uncertainties for the joint unfolded spectrum *except* the impact from unfolding, which are accounted for in the `$A_c$` matrix.

```
plt.imshow(covariance, origin="lower", vmin=-0.001, vmax=0.005);
plt.colorbar();
```

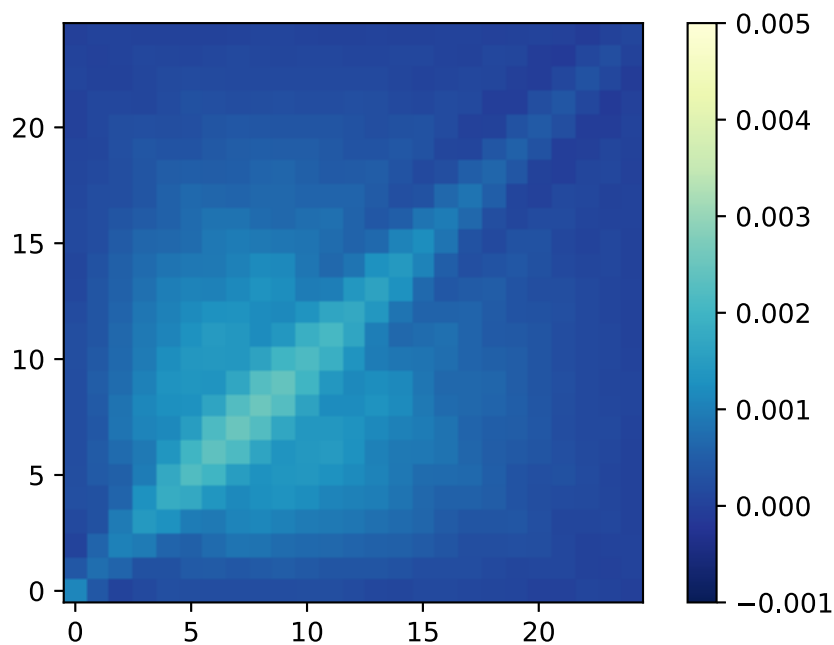

In contrast, the "full covariance" is generated using toy Monte Carlo simulations and includes the uncertainties from unfolding process in addition to the experimental uncertainties.

```
plt.imshow(full_covariance, origin="lower", vmin=-0.001, vmax=0.005);
plt.colorbar();
```

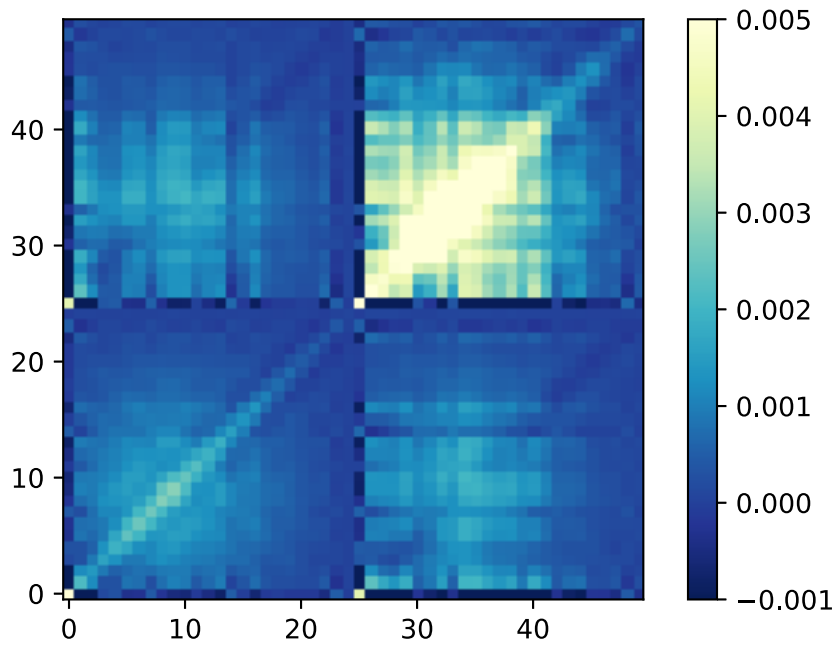

The "diagonal" blocks of this matrix are the uncertainties for  $^{235}\text{U}$  and  $^{239}\text{Pu}$ , while the off-diagonal blocks contain the correlated uncertainties between the two isotopes.

To compare the "full covariance" with the analytic covariance we can focus on the  $^{235}\text{U}$  component of this 50x50 matrix. We then take the square-root of the diagonal elements and divide by the spectrum to generate relative uncertainties, which can be plotted together.

```
full_covariance_u235 = full_covariance[0:25,0:25]

plt.stairs(np.sqrt(np.diagonal(covariance))/spectrum, bin_edges, label='Analytic')
plt.stairs(np.sqrt(np.diagonal(full_covariance_u235))/spectrum, bin_edges, label='Full Covariance')
plt.ylabel('Relative Uncertainty [%]')
plt.xlabel('Antineutrino Energy [MeV]');
plt.ylim(0,0.3)
plt.legend();
```

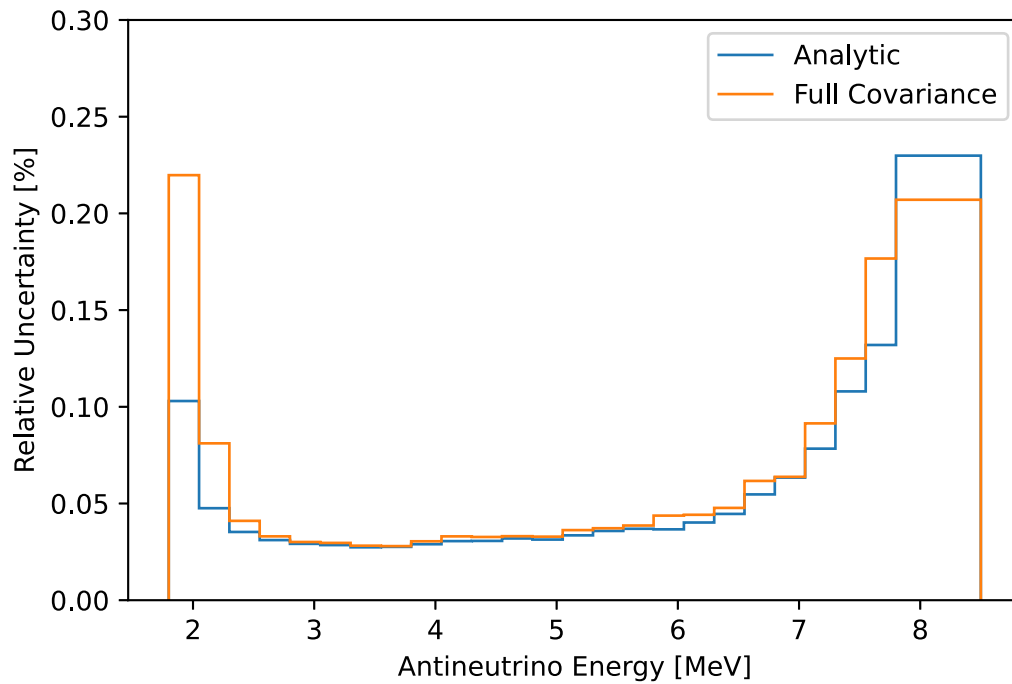

## Model Preparation

For this demonstration we will use the Huber model for  $^{235}\text{U}$  from [Phys.Rev.C84:024617,2011](#), which are available for download ([link](#)). First we need to read the tabulated data for the spectrum of emitted antineutrinos along with the various uncertainties.

```
huber_file = 'U235-anti-neutrino-flux-250keV.dat'

huber_centers = np.loadtxt(huber_file, usecols=0)
huber_235u = np.loadtxt(huber_file, usecols=1)
huber_235u *= 10 # change into same units as measured spectrum
huber_bins = len(huber_235u)

stat_neg = np.loadtxt(huber_file, usecols=2)
stat_pos = np.loadtxt(huber_file, usecols=3)
stat = np.maximum(np.abs(stat_neg), stat_pos)

bias_neg = np.loadtxt(huber_file, usecols=4)
bias_pos = np.loadtxt(huber_file, usecols=5)
bias = np.maximum(np.abs(bias_neg), bias_pos)

z_neg = np.loadtxt(huber_file, usecols=6)
z_pos = np.loadtxt(huber_file, usecols=7)
z_bar = np.maximum(np.abs(z_neg), z_pos)

wm_neg = np.loadtxt(huber_file, usecols=8)
wm_pos = np.loadtxt(huber_file, usecols=9)
wm = np.maximum(np.abs(wm_neg), wm_pos)

norm_neg = np.loadtxt(huber_file, usecols=10)
norm_pos = np.loadtxt(huber_file, usecols=11)
norm = np.maximum(np.abs(norm_neg), norm_pos)
```

The uncertainties as provided by Huber are fractional uncertainties and will need to be multiplied by the spectrum. The statistics and bias uncertainties are fully uncorrelated, so they should be on the diagonal of the covariance matrix. The  $z_{\text{bar}}$ , normalization, and weak magnetism are fully correlated, so they should be throughout the matrix.

```

# Uncorrelated uncertainties get put only on the diagonals.

cov_stat = np.zeros((huber_bins, huber_bins))
for i in range(huber_bins):
    cov_stat[i][i] = stat[i]*stat[i]

cov_bias = np.zeros((huber_bins, huber_bins))
for i in range(huber_bins):
    cov_bias[i][i] = bias[i]*bias[i]

# Correlated uncertainties get spread across all bins:

cov_z_bar = np.zeros((huber_bins, huber_bins))
for i in range(huber_bins):
    for j in range(huber_bins):
        cov_bias[i][j] = z_bar[i]*z_bar[j]

cov_wm = np.zeros((huber_bins, huber_bins))
for i in range(huber_bins):
    for j in range(huber_bins):
        cov_wm[i][j] = wm[i]*wm[j]

cov_norm = np.zeros((huber_bins, huber_bins))
for i in range(huber_bins):
    for j in range(huber_bins):
        cov_norm[i][j] = norm[i]*norm[j]

huber_cov = cov_stat + cov_bias + cov_z_bar + cov_wm + cov_norm

```

Additionally, we will use the Vogel-Beacom IBD cross-section tabulated in [arXiv 1601.06169](#). These data are in 10keV increments, so we will also average the cross-section over each bin width (bin center  $\pm 0.125$  MeV).

```

cross_section_file = 'TCS_CC_anue_p_VB.txt'

xs_e = np.loadtxt(cross_section_file, usecols=0)
xs = np.loadtxt(cross_section_file, usecols=1) * 1e4

n_bins = len(bin_centers)
xs_coarse = np.array([np.average(xs[(xs_e > bin_low[i]) & (xs_e < bin_high[i])]) for i in range(n_bins)])

```

Now we can generate the Huber-predicted  $^{235}\text{U}$  spectrum and interpolate into the experimental binning.

```

# interpolate into experimental binning using exponential interpolation
f = interpolate.interp1d(huber_centers, np.log(huber_235u),
                        kind='linear', fill_value='extrapolate')
u235_model = np.exp(f(bin_centers))

# interpolate errors into experimental binning:
f = interpolate.interp2d(huber_centers, huber_centers,
                        np.log(huber_cov), kind='linear')
model_cov = np.exp(f(bin_centers, bin_centers))

# apply coarse cross-section in experimental binning
u235_model *= xs_coarse

```

```

plt.stairs(u235_model, bin_edges, linewidth=1.3, label='Huber 235U')

plt.stairs(u235_model*(1+np.sqrt(np.diag(model_cov))), bin_edges,
          baseline=u235_model*(1-np.sqrt(np.diag(model_cov))),
          fill=True, color='C0', alpha=0.4)

plt.xlabel('Neutrino Energy [MeV]')
plt.ylabel('Flux x 1e-43')

```

```
plt.legend(loc=1, frameon=True);
plt.ylim(0,2.2);
```

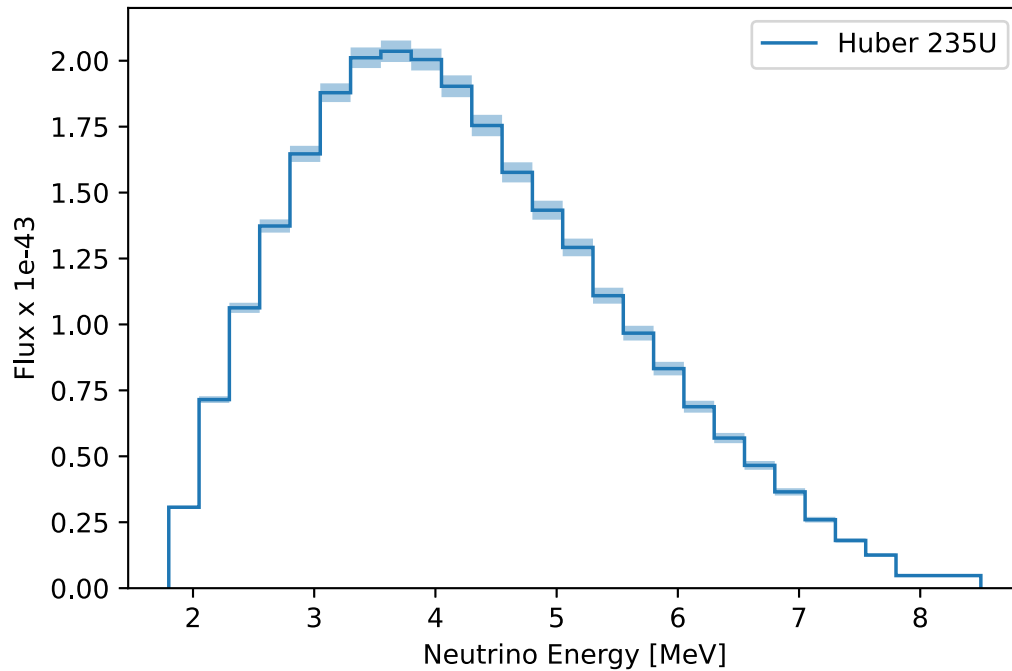

The `A_c` smearing matrix is then applied to a given model to account for smoothing and small bias from the unfolding procedure. We now apply the `A_c` matrix to the Huber model and to the Huber covariance matrix:

```
model_prediction = np.matmul(a_c, u235_model)
model_pred_cov = np.matmul(np.matmul(a_c, model_cov), a_c.T)
```

Comparing the pre- and post-smearing we see that there is a small, but non-zero difference. This highlights the importance of using the `A_c` matrix to account for the impact of unfolding.

```
plt.stairs(u235_model, bin_edges, linewidth=1.3, label='Pre-smearing')
plt.stairs(model_prediction, bin_edges, linewidth=1.3, label='Post-smearing')

plt.xlabel('Neutrino Energy [MeV]');
plt.ylabel('Flux x 1e-43');
plt.legend(loc=1, frameon=True);
plt.ylim(0,2.2);
```

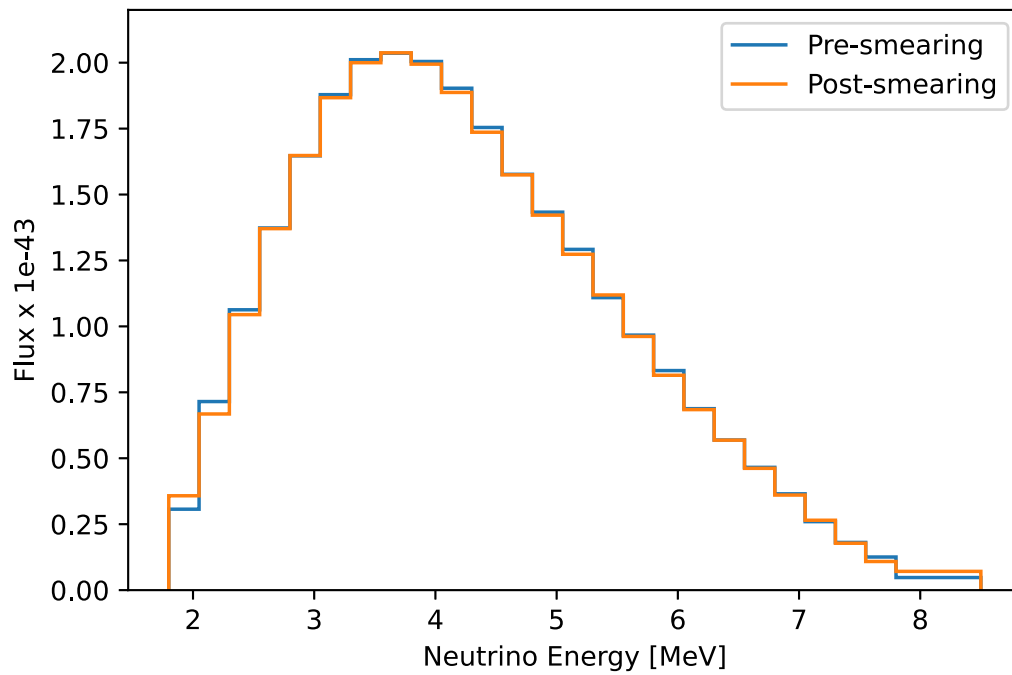

Now we can compare the model prediction (including smearing matrix adjustments) to the unfolded spectrum.

```
plt.stairs(model_prediction, bin_edges,
           linewidth=1.3, label='Huber Prediction')

plt.stairs(model_prediction*(1+np.sqrt(np.diag(model_pred_cov))), bin_edges,
           baseline=model_prediction*(1-np.sqrt(np.diag(model_pred_cov))),
           fill=True, color='C0', alpha=0.4)

plt.errorbar(bin_centers, spectrum, yerr=errorBars,
             marker='.', linestyle='None', label='Unfolded')
plt.xlabel('Neutrino Energy [MeV]');
plt.ylabel('Flux x 1e-43');
plt.legend(loc=1, frameon=True);
plt.ylim(0,2.2);
```



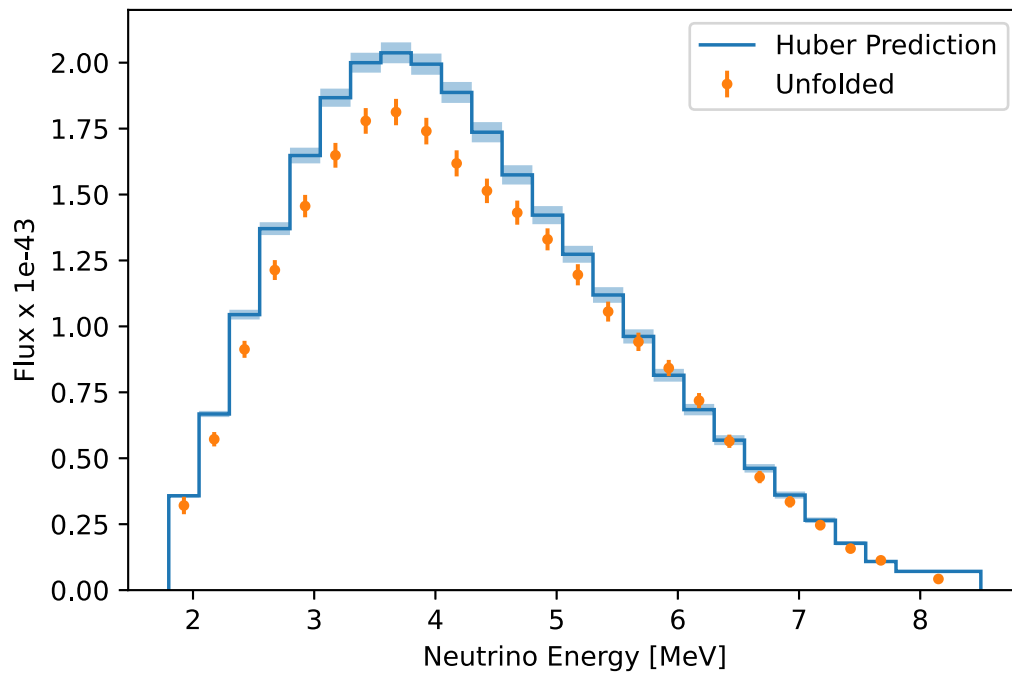

Taking the ratio of the unfolded spectrum to the model prediction we obtain the following comparison:

```
plt.errorbar(bin_centers, spectrum/model_prediction,
             yerr=error_bars/model_prediction, marker='.',
             linestyle='None', label='Data/Model')

plt.plot(bin_centers, np.ones(len(bin_centers)),
         color='k', linestyle='--',
         label='Huber Prediction')

plt.fill_between(bin_centers,
                 np.ones(len(bin_centers))+np.sqrt(np.diag(model_pred_cov)),
                 np.ones(len(bin_centers))-np.sqrt(np.diag(model_pred_cov)),
                 color='k', alpha=0.1, step='mid')
plt.xlabel('Neutrino Energy [MeV]')
plt.ylabel('Ratio (Data/Model)')
plt.ylim(0.5,1.2);
plt.legend(loc=3, frameon=True);
```

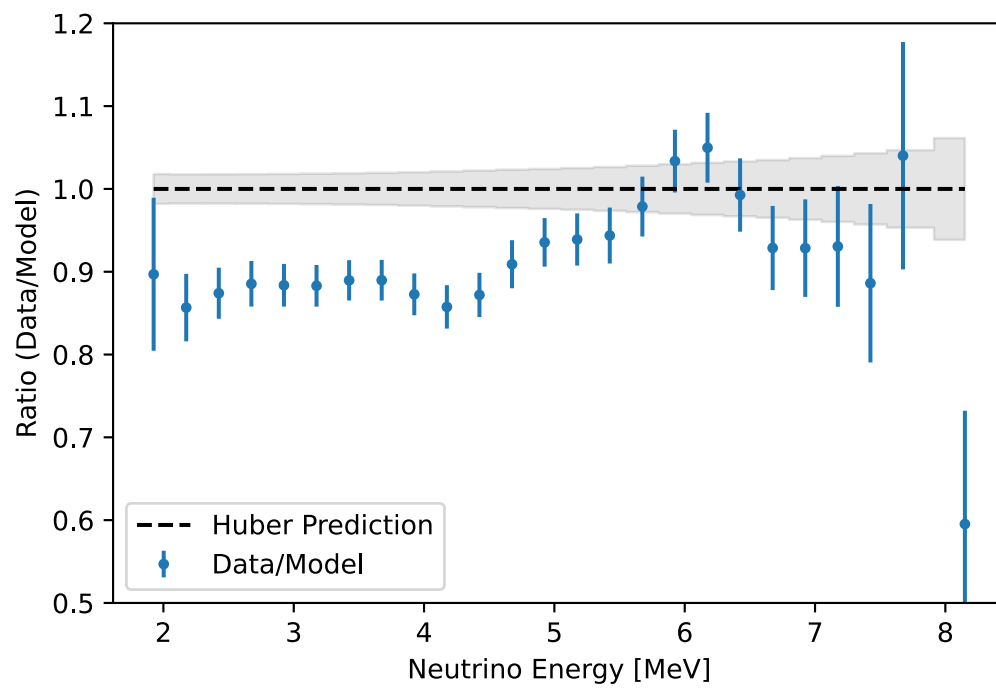

## Summary

Here we have demonstrated how to read and use the supplemental material provided alongside this manuscript. We have made an example comparison to the Huber model for  $^{235}\text{U}$  that can be a template for comparing to any model of choice.
